# Supplementary material for: Better May Not Be Fairer: A Study on Subgroup Discrepancy in Image Classification
Source: arXiv:2212.08649 source file (2023-09-22)
Supplement: Supplementary file 1 [file appendix.tex]

\section{Appendix}

\begin{table*}
 \centering
  \begin{adjustbox}{max width=\textwidth}
  \begin{tabular}{lcc}
    \toprule
      & CIFAR10-C & CIFAR100-C \\
     \midrule
    Baseline & 90.44/90.38 &67.84/67.84\\
    Mixup    & 92.71/92.54 &69.47/68.69\\
    Cutout   & 90.27/90.15 &65.32/65.29  \\
    Cutmix   & 90.31/90.23 &67.05/66.61  \\
    AutoAug  & 92.87/92.81 &71.8/71.25 \\
    \midrule
    Ours (Trunc Gaussian on $\nu$) & 90.77/90.77 & 68.03/67.93 \\
    Ours (Mix $\nu$) & 87.94/87.13 & 63.15/60.06 \\
    Ours (Mix $z$) & 90.79/90.42 &66.15/65.56  \\
    + Std & 90.45/90.47 &67.29/67.16 \\
    Ours (Uniform on $z$)  & 91.33/91.3 &69.36/69.38 \\
    Ours (Trunc Gaussian on $z$) & 91.52/91.49 &69.24/69.25\\
    + Std & 91.1/91.27 &69.2/69.07 \\
    + Std + Mix $z$ & 91.31/91 &69.01/69.05\\
    \bottomrule
  \end{tabular}
  \end{adjustbox}
  \caption{\textbf{Cifar10-C and Cifar100-C.} }
  \label{tab:cifarc}
\end{table*}
